# Supplementary material for: Structure-imposed electronic topology in cove-edged graphene nanoribbons
Source: arXiv:2205.15811 source file (2022-11-22)
Supplement: Supplementary file 1 [file SM.pdf]

# Structure-imposed electronic topology in cove-edged graphene nanoribbons - Supplemental Material

Florian M. Arnold,<sup>1,\*</sup> Tsai-Jung Liu,<sup>1,\*</sup> Agnieszka Kuc,<sup>2</sup> and Thomas Heine<sup>1,2,3,†</sup>

<sup>1</sup>*Faculty of Chemistry and Food Chemistry,*

*TU Dresden, Bergstrasse 66c, 01069 Dresden, Germany*

<sup>2</sup>*Helmholtz-Zentrum Dresden-Rossendorf, Institute of Resource Ecology,*

*Permoserstrasse 15, 04318 Leipzig, Germany*

<sup>3</sup>*Department of Chemistry, Yonsei University,*

*Seodaemun-gu, Seoul 120-749, Republic of Korea*

This supplemental material contains:

- Fig. S1, showing ZGNR-C with widths  $N = 4 \dots 7$  as examples for the nomenclature of cove-edged ZGNR. For each structure the symmetry elements and the Frieze group are included.
- Section S1, detail information on tight-binding calculations.
- Fig. S2, giving tables of  $\mathbb{Z}_2$  for an extended set of ZGNR-C, similar to Fig. 2(a-d).
- Fig. S3, showing a set of exemplary band structures with a direct band gap at  $k = \pi$  if  $a$  is even (4-ZGNR-C(2,0)), at  $k = 0$  if  $a$  is odd (4-ZGNR-C(3,0)), or metallic if  $b = \frac{a}{2}$ .
- Fig. S4, visualizing the fit results given in Eq. (10) and demonstrating the behavior of the band gap for large  $N$ , testing the validity of the fit for  $\Delta_{\max}$ .
- Fig. S5, giving tables of realized termination types for an extended set of ZGNR-C with both  $\mathbf{S}$  and  $\mathbf{L}$  as reference points at the boundary, similar to Fig. 5.
- Fig. S6, containing a scheme for the realized termination types of ZGNR-C.

---

\* Equal contribution

† thomas.heine@tu-dresden.de

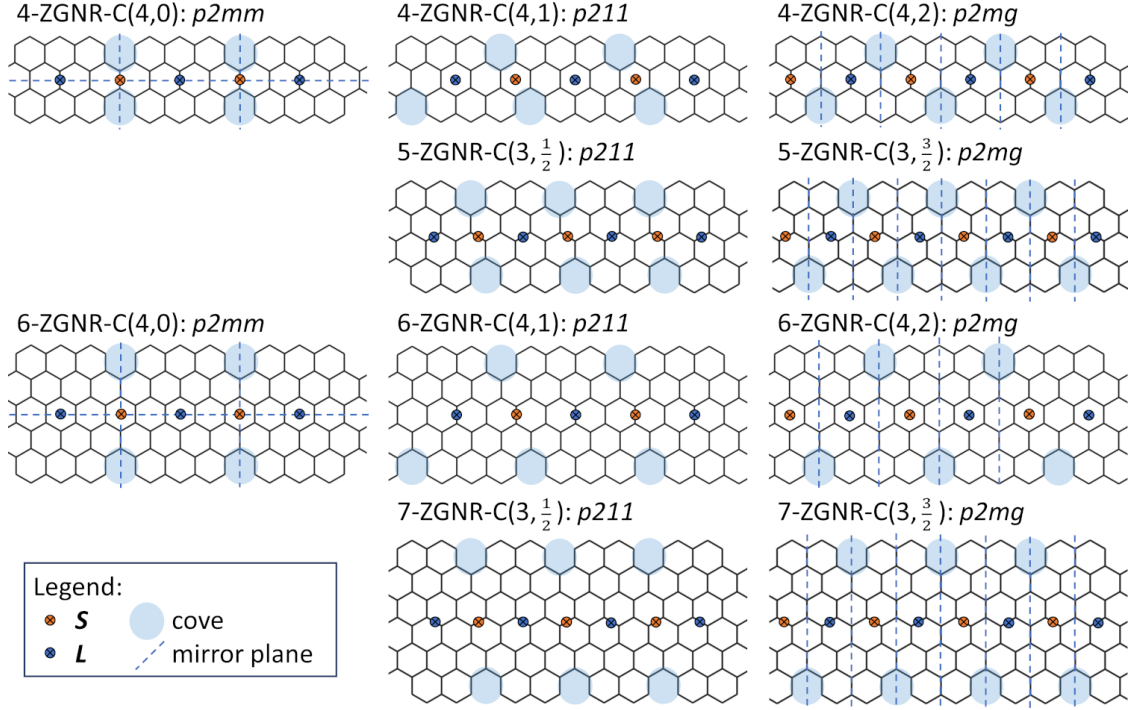

FIG. S1. Representative ZGNR-C structures with widths  $N = 4 \dots 7$ . The respective label, the Frieze group and the relevant symmetry elements are indicated for each structure.

## S1. TIGHT-BINDING (TB) CALCULATION DETAILS

Throughout this paper, the `pythTB` package, which can be downloaded from <http://www.physics.rutgers.edu/pythtb/>, is used. In this package, `pythtb.tb_model` class is the main tight-binding model class. Dimensionality, orbitals, lattice vectors, on-site energies and hopping parameters can be set up with this class. Here, only one  $\pi$ -electron per carbon atom is considered with 1<sup>st</sup>-neighbor interaction  $t_1 = -1$ . To satisfy the symmetry requirement, real-space origin is placed at the center of the cell, which is also an inversion center for ZGNR-C. In this class, band structure can be calculated with given path and k-grid.

`pythtb.wf_array` is a class designed for calculating topological properties. With `solve_on_grid` function solving the TB model at each grid point within the BZ, and `berry_phase` function doing the numerical integration for all occupied bands, Zak phase is obtained for 1D system.

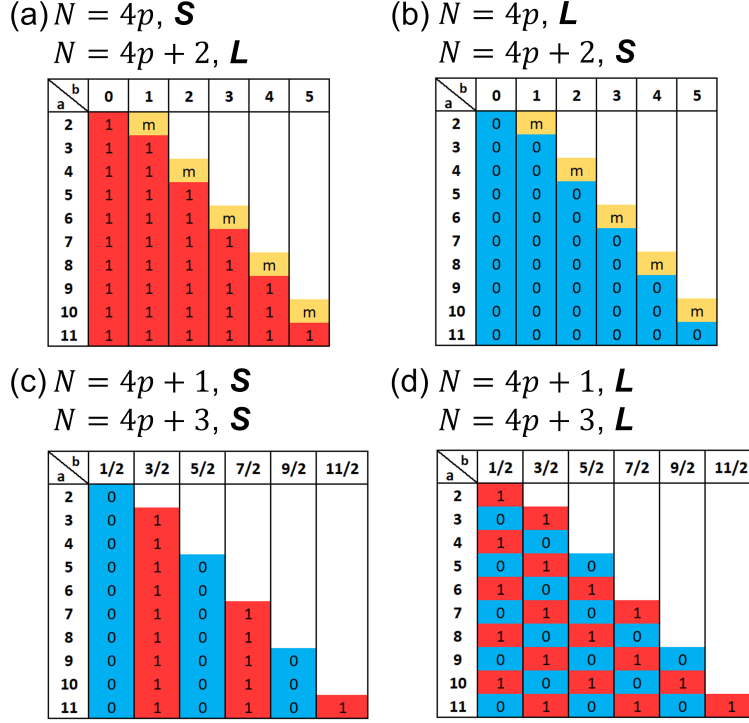

FIG. S2.  $\mathbb{Z}_2$  invariant for ZGNR-C: (a)  $N = 4p$  (with integer  $p = 1, 2, \dots$ ) with  $\mathbf{S}$  or  $N = 4p + 2$  with  $\mathbf{L}$  at the boundary, (b)  $N = 4p$  with  $\mathbf{L}$  or  $N = 4p + 2$  with  $\mathbf{S}$  at the boundary, (c)  $N = 4p + 1$  and  $N = 4p + 3$  with  $\mathbf{S}$  and (d)  $N = 4p + 1$  and  $N = 4p + 3$  with  $\mathbf{L}$  at the boundary. Structure parameters  $a$  and  $b$  are varied in rows and columns, respectively, with  $a \leq 11$ . Topological insulators ( $\mathbb{Z}_2 = 1$ ) are marked in red, trivial semiconductors ( $\mathbb{Z}_2 = 0$ ) in blue, metallic ribbons are indicated as "m" (yellow).

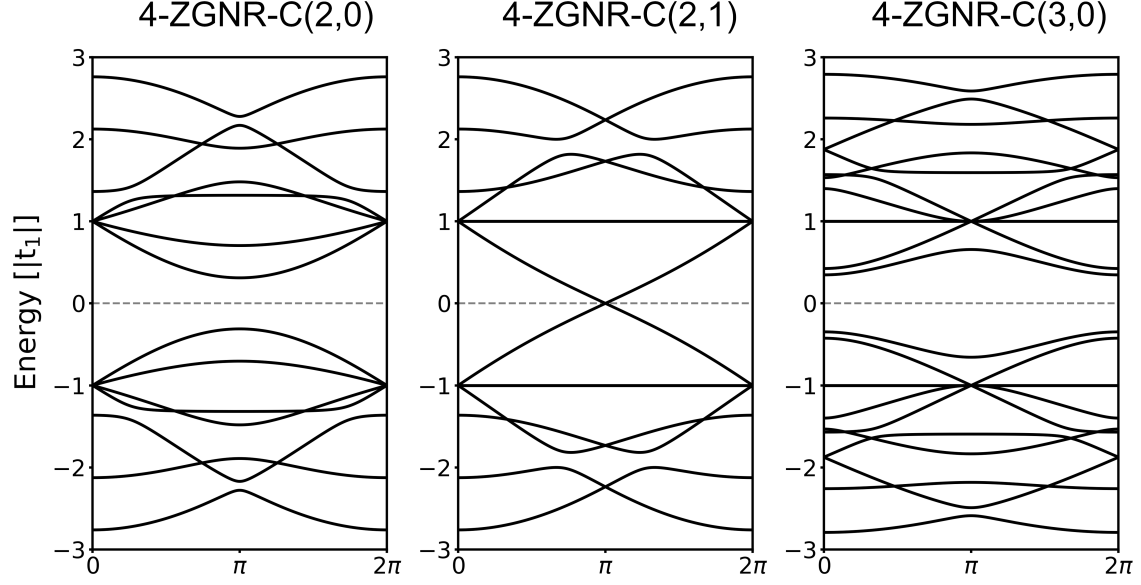

FIG. S3. Electronic band structures for 4-ZGNR-C(2,0), 4-ZGNR-C(2,1), and 4-ZGNR-C(3,0) calculated by TB.

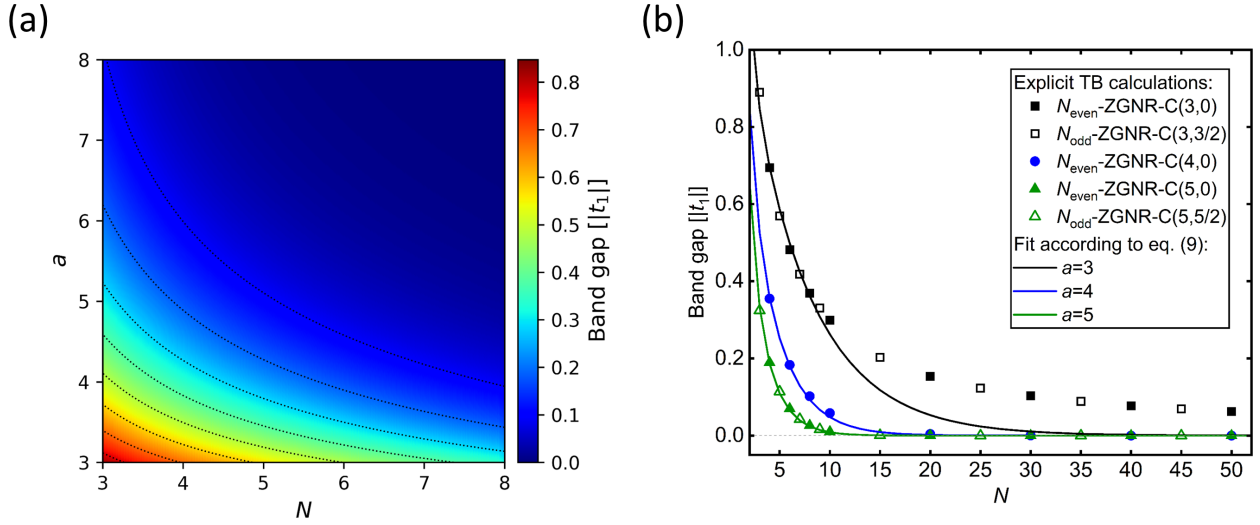

FIG. S4. (a) Estimated  $\Delta_{\max}$  as function of  $N$  and  $a$  according to Eq. (10). Dashed lines are isolines of  $\Delta_{\max}$  with  $0.1 |t_1|$  difference between each other. (b) Electronic band gap for large  $N$ , demonstrated using exemplary structures and curves obtained for the chosen  $a$  using Eq. (10).

(a)  $N = 4p, \alpha = 60^\circ, 120^\circ, \mathbf{S}$  (b)  $N = 4p + 2, \alpha = 60^\circ, 120^\circ, \mathbf{S}$

| $\begin{smallmatrix} b \\ a \end{smallmatrix}$ | 0  | 1  | 2  | 3  | 4  | 5  |
|------------------------------------------------|----|----|----|----|----|----|
| 2                                              | bd | zz |    |    |    |    |
| 3                                              | bd | zz |    |    |    |    |
| 4                                              | bd | zz | bd |    |    |    |
| 5                                              | bd | zz | bd |    |    |    |
| 6                                              | bd | zz | bd | zz |    |    |
| 7                                              | bd | zz | bd | zz |    |    |
| 8                                              | bd | zz | bd | zz | bd |    |
| 9                                              | bd | zz | bd | zz | bd |    |
| 10                                             | bd | zz | bd | zz | bd | zz |
| 11                                             | bd | zz | bd | zz | bd | zz |

| $\begin{smallmatrix} b \\ a \end{smallmatrix}$ | 0  | 1  | 2  | 3  | 4  | 5  |
|------------------------------------------------|----|----|----|----|----|----|
| 2                                              | zz | bd |    |    |    |    |
| 3                                              | zz | bd |    |    |    |    |
| 4                                              | zz | bd | zz |    |    |    |
| 5                                              | zz | bd | zz |    |    |    |
| 6                                              | zz | bd | zz | bd |    |    |
| 7                                              | zz | bd | zz | bd |    |    |
| 8                                              | zz | bd | zz | bd | zz |    |
| 9                                              | zz | bd | zz | bd | zz |    |
| 10                                             | zz | bd | zz | bd | zz | bd |
| 11                                             | zz | bd | zz | bd | zz | bd |

(c)  $N = 4p + 1, \alpha = 60^\circ, \mathbf{S}$

| $\begin{smallmatrix} b \\ a \end{smallmatrix}$ | 1/2 | 3/2 | 5/2 | 7/2 | 9/2 | 11/2 |
|------------------------------------------------|-----|-----|-----|-----|-----|------|
| 2                                              | zz  |     |     |     |     |      |
| 3                                              | zz  | bd  |     |     |     |      |
| 4                                              | zz  | bd  |     |     |     |      |
| 5                                              | zz  | bd  | zz  |     |     |      |
| 6                                              | zz  | bd  | zz  |     |     |      |
| 7                                              | zz  | bd  | zz  | bd  |     |      |
| 8                                              | zz  | bd  | zz  | bd  |     |      |
| 9                                              | zz  | bd  | zz  | bd  | zz  |      |
| 10                                             | zz  | bd  | zz  | bd  | zz  |      |
| 11                                             | zz  | bd  | zz  | bd  | zz  | bd   |

(d)  $N = 4p + 1, \alpha = 120^\circ, \mathbf{S}$

| $\begin{smallmatrix} b \\ a \end{smallmatrix}$ | 1/2 | 3/2 | 5/2 | 7/2 | 9/2 | 11/2 |
|------------------------------------------------|-----|-----|-----|-----|-----|------|
| 2                                              | bd  |     |     |     |     |      |
| 3                                              | bd  | zz  |     |     |     |      |
| 4                                              | bd  | zz  |     |     |     |      |
| 5                                              | bd  | zz  | bd  |     |     |      |
| 6                                              | bd  | zz  | bd  |     |     |      |
| 7                                              | bd  | zz  | bd  | zz  |     |      |
| 8                                              | bd  | zz  | bd  | zz  |     |      |
| 9                                              | bd  | zz  | bd  | zz  | bd  |      |
| 10                                             | bd  | zz  | bd  | zz  | bd  |      |
| 11                                             | bd  | zz  | bd  | zz  | bd  | zz   |

(e)  $N = 4p, \alpha = 60^\circ, 120^\circ, \mathbf{L}$

| $\begin{smallmatrix} b \\ a \end{smallmatrix}$ | 0  | 1  | 2  | 3  | 4  | 5  |
|------------------------------------------------|----|----|----|----|----|----|
| 2                                              | bd | zz |    |    |    |    |
| 3                                              | zz | bd |    |    |    |    |
| 4                                              | bd | zz | bd |    |    |    |
| 5                                              | zz | bd | zz |    |    |    |
| 6                                              | bd | zz | bd | zz |    |    |
| 7                                              | zz | bd | zz | bd |    |    |
| 8                                              | bd | zz | bd | zz | bd |    |
| 9                                              | zz | bd | zz | bd | zz |    |
| 10                                             | bd | zz | bd | zz | bd | zz |
| 11                                             | zz | bd | zz | bd | zz | bd |

(f)  $N = 4p + 2, \alpha = 60^\circ, 120^\circ, \mathbf{L}$

| $\begin{smallmatrix} b \\ a \end{smallmatrix}$ | 0  | 1  | 2  | 3  | 4  | 5  |
|------------------------------------------------|----|----|----|----|----|----|
| 2                                              | zz | bd |    |    |    |    |
| 3                                              | bd | zz |    |    |    |    |
| 4                                              | zz | bd | zz |    |    |    |
| 5                                              | bd | zz | bd |    |    |    |
| 6                                              | zz | bd | zz | bd |    |    |
| 7                                              | bd | zz | bd | zz |    |    |
| 8                                              | zz | bd | zz | bd | zz |    |
| 9                                              | bd | zz | bd | zz | bd |    |
| 10                                             | zz | bd | zz | bd | zz | bd |
| 11                                             | bd | zz | bd | zz | bd | zz |

(g)  $N = 4p + 1, \alpha = 60^\circ, \mathbf{L}$

| $\begin{smallmatrix} b \\ a \end{smallmatrix}$ | 1/2 | 3/2 | 5/2 | 7/2 | 9/2 | 11/2 |
|------------------------------------------------|-----|-----|-----|-----|-----|------|
| 2                                              | zz  |     |     |     |     |      |
| 3                                              | bd  | zz  |     |     |     |      |
| 4                                              | zz  | bd  |     |     |     |      |
| 5                                              | bd  | zz  | bd  |     |     |      |
| 6                                              | zz  | bd  | zz  |     |     |      |
| 7                                              | bd  | zz  | bd  | zz  |     |      |
| 8                                              | zz  | bd  | zz  | bd  |     |      |
| 9                                              | bd  | zz  | bd  | zz  | bd  |      |
| 10                                             | zz  | bd  | zz  | bd  | zz  |      |
| 11                                             | bd  | zz  | bd  | zz  | bd  | zz   |

(h)  $N = 4p + 1, \alpha = 120^\circ, \mathbf{L}$

| $\begin{smallmatrix} b \\ a \end{smallmatrix}$ | 1/2 | 3/2 | 5/2 | 7/2 | 9/2 | 11/2 |
|------------------------------------------------|-----|-----|-----|-----|-----|------|
| 2                                              | bd  |     |     |     |     |      |
| 3                                              | zz  | bd  |     |     |     |      |
| 4                                              | bd  | zz  |     |     |     |      |
| 5                                              | zz  | bd  | zz  |     |     |      |
| 6                                              | bd  | zz  | bd  |     |     |      |
| 7                                              | zz  | bd  | zz  | bd  |     |      |
| 8                                              | bd  | zz  | bd  | zz  |     |      |
| 9                                              | zz  | bd  | zz  | bd  | zz  |      |
| 10                                             | bd  | zz  | bd  | zz  | bd  |      |
| 11                                             | zz  | bd  | zz  | bd  | zz  | bd   |

FIG. S5. Termination types for ZGNR-C: (a-d) Unit cells with  $\mathbf{S}$  at the boundary with (a)  $N = 4p$  and (b)  $N = 4p + 2$  for both  $\alpha = 60^\circ$  and  $\alpha = 120^\circ$ , (c)  $N = 4p + 1, \alpha = 60^\circ$  or  $N = 4p + 3, \alpha = 120^\circ$  and (d)  $N = 4p + 1, \alpha = 120^\circ$  or  $N = 4p + 3, \alpha = 60^\circ$ . (e-h) Unit cells with  $\mathbf{L}$  at the boundary with (e)  $N = 4p$  and (f)  $N = 4p + 2$  for both  $\alpha = 60^\circ$  and  $\alpha = 120^\circ$ , (g)  $N = 4p + 1, \alpha = 60^\circ$  or  $N = 4p + 3, \alpha = 120^\circ$  and (h)  $N = 4p + 1, \alpha = 120^\circ$  or  $N = 4p + 3, \alpha = 60^\circ$ . Zigzag terminations are indicated by labels "zz" in orange, and bearded by "bd" in blue.

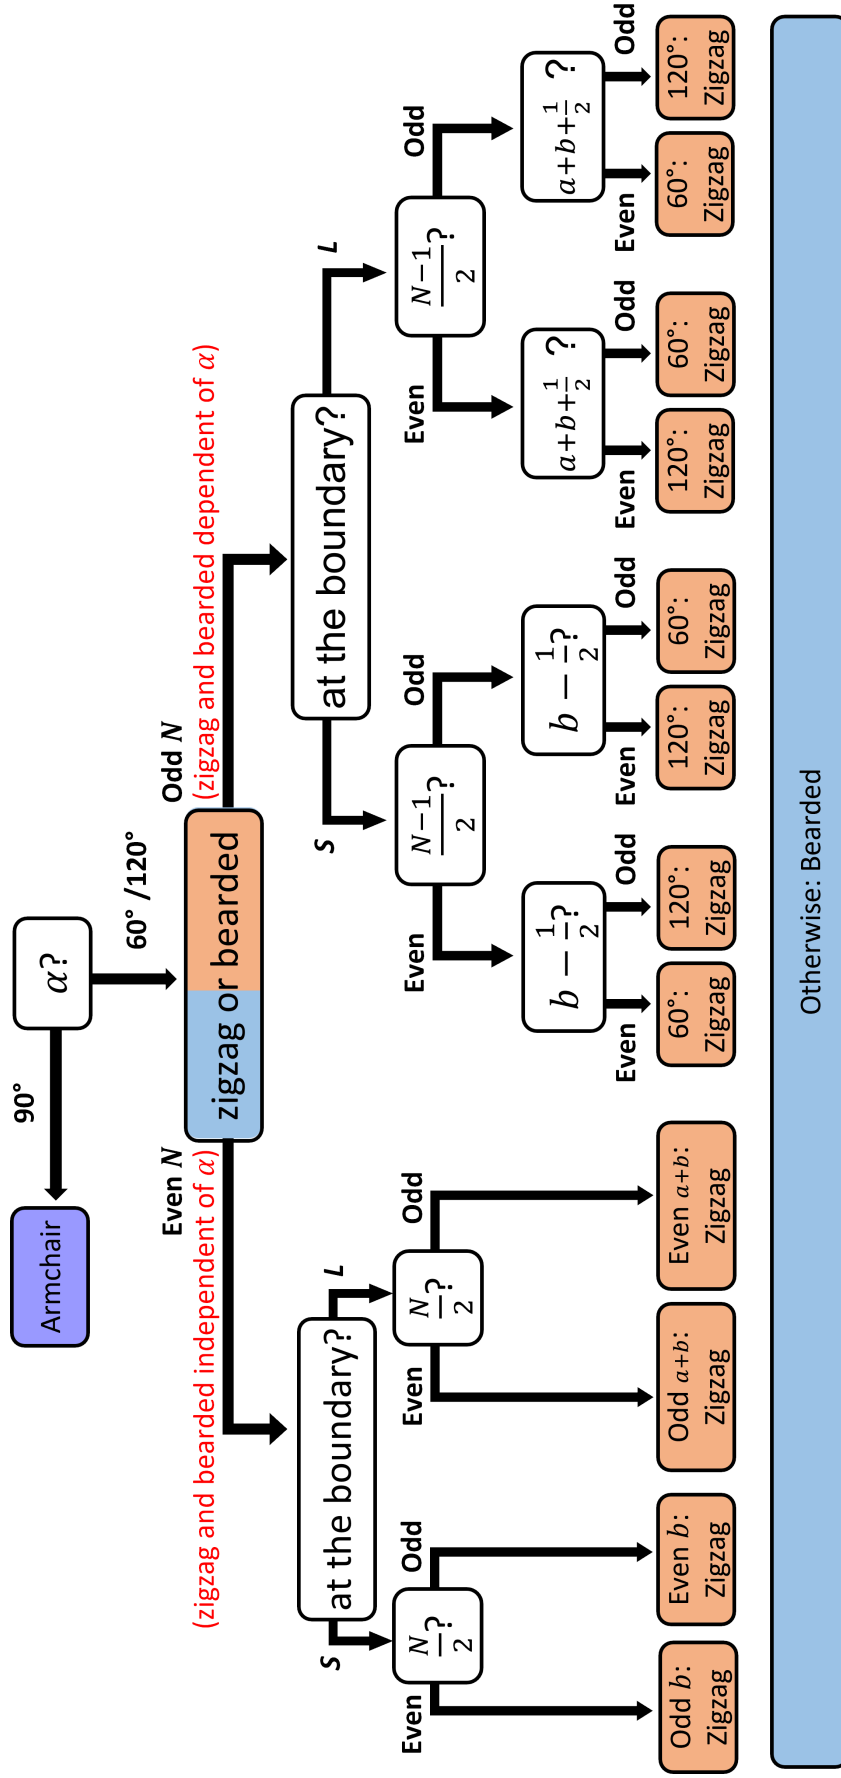

FIG. S6. Scheme for realized termination types in ZGNR-C.
